# Supplementary material for: Scalable Semantic Non-Markovian Simulation Proxy for Reinforcement Learning
Source: arXiv:2310.06835 source file (2023-10-15)
Supplement: Supplementary file 1 [file iaai_si.tex]

\section{Longer Explainable Trace}

\section{Step by step play through of a single episode}
Follow Deep Symbolic Policy Learning paper from class - videos and some writing in supplement.

\section{Base policy for Blue agent}

\section{An introduction to Pyreason-gym}
